# Supplementary material for: FlowAct-R1: Towards Interactive Humanoid Video Generation
Source: arXiv:2601.10103 source file (2026-01-15)
Supplement: Supplementary file 1 [file appendix.tex]

\section{Hello World}
%\subsection{Hello World}
